# Supplementary material for: Can LLMs Learn by Teaching for Better Reasoning? A Preliminary Study
Source: arXiv:2406.14629 source file (2024-11-24)
Supplement: Supplementary file 1 [file EA.tex]

class Solution():
    def winnerSquareGame(self, n: int) -> bool:
        squares = set(i * i for i in range(int(math.sqrt(n)) + 1))
        memo = {}

        def canWin(n: int) -> bool:
            if n <= 0:
                return False
            if n in memo:
                return memo[n]
            for square in squares:
                if square > n:
                    break
                if not canWin(n - square):
                    memo[n] = True
                    return True
            memo[n] = False
            return False

        return canWin(n)
