# Supplementary material for: Can LLMs Learn by Teaching for Better Reasoning? A Preliminary Study
Source: arXiv:2406.14629 source file (2024-11-24)
Supplement: Supplementary file 2 [file TA.tex]

from typing import List

class Solution():
    def predictTheWinner(self, nums: List[int]) -> bool:
        n = len(nums)
        dp = [[0] * n for _ in range(n)]

        def calculateScores(start: int, end: int) -> int:
            if start > end:
                return 0
            if dp[start][end] != 0:
                return dp[start][end]
            
            chooseStart = nums[start] - calculateScores(start + 1, end)
            chooseEnd = nums[end] - calculateScores(start, end - 1)
            
            dp[start][end] = max(chooseStart, chooseEnd)
            
            return dp[start][end]
        
        return calculateScores(0, n - 1) >= 0
