# Supplementary material for: Can LLMs Learn by Teaching for Better Reasoning? A Preliminary Study
Source: arXiv:2406.14629 source file (2024-11-24)
Supplement: Supplementary file 3 [file EA.tex]

from typing import List

class Solution():
    def predictTheWinner(self, nums: List[int]) -> bool:
        def dfs(start: int, end: int) -> int:
            if start > end:
                return 0
            
            chooseStart = nums[start] - dfs(start + 1, end)
            chooseEnd = nums[end] - dfs(start, end - 1)
            
            return max(chooseStart, chooseEnd)
        
        scoreDiff = dfs(0, len(nums) - 1)
        return scoreDiff >= 0
