# Supplementary material for: Can LLMs Learn by Teaching for Better Reasoning? A Preliminary Study
Source: arXiv:2406.14629 source file (2024-11-24)
Supplement: Supplementary file 4 [file TA.tex]

from typing import List

class Solution():
    def stoneGameIII(self, stoneValue: List[int]) -> str:
        def dfs(i: int, stoneValues: List[int]) -> int:
            if i >= len(stoneValues):
                return 0
            
            maxScore = float('-inf')
            for j in range(i, min(i+3, len(stoneValues))):
                currScore = sum(stoneValues[i:j+1])
                opponentScoreDiff = dfs(j + 1, stoneValues)
                maxScore = max(maxScore, currScore - opponentScoreDiff)
                
            return maxScore
        
        scoreDiff = dfs(0, stoneValue)
        if scoreDiff > 0:
            return 'Alice'
        elif scoreDiff < 0:
            return 'Bob'
        else:
            return 'Tie'
