# Supplementary material for: Can LLMs Learn by Teaching for Better Reasoning? A Preliminary Study
Source: arXiv:2406.14629 source file (2024-11-24)
Supplement: Supplementary file 5 [file EA.tex]

from typing import List

class Solution():
    def stoneGameIII(self, stoneValue: List[int]) -> str:
        n = len(stoneValue)
        scores = [0] * (n + 1)
        
        for i in range(n-1, -1, -1):
            take1 = stoneValue[i] - scores[i+1]
            |take2 = sum(stoneValue[i:i+2]) - scores[i+2] if i+2 <= n else float('-inf')
            take3 = sum(stoneValue[i:i+3]) - scores[i+3] if i+3 <= n else float('-inf')|
            scores[i] = max(take1, take2, take3)
            
        if scores[0] > sum(stoneValue) - scores[0]:
            return "Alice"
        elif scores[0] < sum(stoneValue) - scores[0]:
            return "Bob"
        else:
            return "Tie"
