# Supplementary material for: Can LLMs Learn by Teaching for Better Reasoning? A Preliminary Study
Source: arXiv:2406.14629 source file (2024-11-24)
Supplement: Supplementary file 8 [file TA.tex]

from typing import List

class Solution:
    def predictTheWinner(self, nums: List[int]) -> bool:
        n = len(nums)
        dp1, dp2 = [0] * n, [0] * n
        dp1[0], dp2[0] = nums[0], 0
        for i in range(1, n):
            dp1[i] = max(dp1[i-1] + nums[i], dp2[i-1])
            dp2[i] = max(dp1[i-1], dp2[i-1] + nums[i])
        return dp1[-1] > dp2[-1]
