# Supplementary material for: Can LLMs Learn by Teaching for Better Reasoning? A Preliminary Study
Source: arXiv:2406.14629 source file (2024-11-24)
Supplement: Supplementary file 9 [file EA.tex]

from typing import List

class Solution:
    def stoneGame(self, piles: List[int]) -> bool:
        n = len(piles)
        prefix_sum = [0] * (n + 1)
        for i in range(n):
            prefix_sum[i + 1] = prefix_sum[i] + piles[i]
        
        def dp(i, j):
            if i > j:
                return 0
            return max(piles[i - 1] + prefix_sum[j] - prefix_sum[i] - dp(i + 1, j), 
                       piles[j] + prefix_sum[i] - prefix_sum[j - 1] - dp(i, j - 1))
        
        return dp(1, n) \% 2 == 1
