# Supplementary material for: Can LLMs Learn by Teaching for Better Reasoning? A Preliminary Study
Source: arXiv:2406.14629 source file (2024-11-24)
Supplement: Supplementary file 12 [file EA.tex]

from typing import List

class Solution:
    def predictTheWinner(self, nums: List[int]) -> bool:
        n = len(nums)
        dp = [[0] * n for _ in range(n)]

        # Base case: diagonal elements
        for i in range(n):
            dp[i][i] = nums[i]

        # Dynamic programming iteration
        for length in range(2, n+1):
            for i in range(n - length + 1):
                j = i + length - 1
                dp[i][j] = max(nums[i] - dp[i+1][j], nums[j] - dp[i][j-1])

        # Return the result
        return dp[0][n-1] >= 0
