# Supplementary material for: Can LLMs Learn by Teaching for Better Reasoning? A Preliminary Study
Source: arXiv:2406.14629 source file (2024-11-24)
Supplement: Supplementary file 13 [file TA.tex]

from typing import List
  
class Solution:
  def stoneGame(self, piles: List[int]) -> bool:
    n = len(piles)
    dp = [[0] * n for _ in range(n)]

    # Base case: diagonal elements
    for i in range(n):
        dp[i][i] = piles[i]

    # Dynamic programming iteration
    for length in range(2, n+1):
        for i in range(n - length + 1):
            j = i + length - 1
            dp[i][j] = max(piles[i] - dp[i+1][j], piles[j] - dp[i][j-1])

    # Return the winner
    return dp[0][n-1] > 0
