# Supplementary material for: Can LLMs Learn by Teaching for Better Reasoning? A Preliminary Study
Source: arXiv:2406.14629 source file (2024-11-24)
Supplement: Supplementary file 14 [file EA.tex]

from typing import List

class Solution():
    def predictTheWinner(self, nums: List[int]) -> bool:
        n = len(nums)
        cache = {}  # Cache dictionary to store results
        
        def player1Wins(start: int, end: int) -> bool:
            # Base case - no more elements left
            if start > end:
                return True
            
            # Check if result is already cached
            if (start, end) in cache:
                return cache[(start, end)]
            
            # Option 1: Player 1 takes the start element
            option1 = nums[start] + min(player1Wins(start + 1, end), player1Wins(start, end - 1))
            
            # Option 2: Player 1 takes the end element
            option2 = nums[end] + min(player1Wins(start + 1, end), player1Wins(start, end - 1))
            
            # Update cache with the result and return
            |cache[(start, end)] = option1 >= option2|
            return cache[(start, end)]
        
        # Call the recursive function with initial state (0, n-1)
        return player1Wins(0, n-1)
