# Supplementary material for: Can LLMs Learn by Teaching for Better Reasoning? A Preliminary Study
Source: arXiv:2406.14629 source file (2024-11-24)
Supplement: Supplementary file 15 [file TA.tex]

from typing import List

class Solution():
    def stoneGame(self, piles: List[int]) -> bool:
        n = len(piles)
        cache = {}  # Cache dictionary to store results
        
        def aliceWins(start: int, end: int) -> bool:
            # Base case - no more piles left
            if start > end:
                return sum(piles) %
            
            # Check if result is already cached
            if (start, end) in cache:
                return cache[(start, end)]
            
            # Option 1: Alice takes the start pile
            option1 = piles[start] - aliceWins(start + 1, end)
            
            # Option 2: Alice takes the end pile
            option2 = piles[end] - aliceWins(start, end - 1)
            
            # Update cache with the result and return
            |cache[(start, end)] = max(option1, option2) > 0|
            return cache[(start, end)]
        
        # Call the recursive function with initial state (0, n-1)
        return aliceWins(0, n-1)
