# Supplementary material for: Can LLMs Learn by Teaching for Better Reasoning? A Preliminary Study
Source: arXiv:2406.14629 source file (2024-11-24)
Supplement: Supplementary file 16 [file EA.tex]

from typing import List

class Solution():
    def predictTheWinner(self, nums: List[int]) -> bool:
        total_elements = len(nums)
        
        if total_elements %
            return True
        else:
            return sum(nums) >= sum(nums) // 2
