# Supplementary material for: Can LLMs Learn by Teaching for Better Reasoning? A Preliminary Study
Source: arXiv:2406.14629 source file (2024-11-24)
Supplement: Supplementary file 17 [file TA.tex]

from typing import List

class Solution():
    def stoneGame(self, piles: List[int]) -> bool:
        total_stones = sum(piles)
        half_total = total_stones // 2
        
        if half_total <= max(piles):
            return True
        else:
            return False
